# Supplementary material for: Is Graph Convolution Always Beneficial For Every Feature?
Source: arXiv:2411.07663 source file (2024-11-12)
Supplement: Supplementary file 1 [file datasets_license.tex]

\begin{table}[htbp]
\centering
\begin{tabular}{*{2}{c}}
\toprule
\textbf{Dataset} & \textbf{License}\\
\midrule
Children & MIT license \\
Computers & MIT license \\
Fitness & MIT license \\
History & MIT license \\
Photo & MIT license \\
Amazon-Ratings & MIT license \\
Minesweeper & MIT license \\
Questions & MIT license \\
Roman-Empire & MIT license \\
Tolokers & MIT license \\
\bottomrule
\end{tabular}
\caption{The License of Datasets}
\label{tab:apd_datasets_license}
\end{table}
